# Supplementary material for: HowkGPT: Investigating the Detection of ChatGPT-generated University Student Homework through Context-Aware Perplexity Analysis
Source: arXiv:2305.18226 source file (2025-03-11)
Supplement: Supplementary file 1 [file 100_appendix.tex]

\begin{table*}[!t]
\caption{A sample question and corresponding responses from a randomly selected student and ChatGPT.}
\label{table:QandA}
\centering
\begin{tabular}{ |p{0.98\textwidth}| }
\hline
\textbf{Question: }
\textit{This question seeks information about today’s cyber-threat landscape. In a few paragraphs, please describe the types of cyber-threats available, and also describe the motivation behind using cyber-attacks instead of physical attacks.} \\
\hline
\textbf{Student: }
With the rise of the IoT and crypto industries, the development of AI and machine learning, and frankly, the inescapable digitalization of every aspect of our lives, the digital world finds itself in a rather troubling situation. There are various cyber threats that pose threat to computer systems nowadays and it does not seem that their number is going to diminish. Cyber worms, botnets, rootkits and backdoors, different types of ransomwares, DDoS attacks, spam, and phishing (especially email phishing), trojans, backdoors, etc. – all the after-mentioned vulnerabilities pose a tremendous threat to computer systems. In our readings, we have extensively covered some infamous examples of such vulnerabilities: the
Stuxnet cyber worm which was used to attack Nantanz nuclear facility in Iran, the Mirai botnet, which was utilized to primarily attack IoT devices in targeted regions worldwide, WannaCry and Petya ransomware (that used EternalBlue and DoublePulsar exploits) and infected hundreds of thousands of systems, and many others.
Cybercriminals may utilize various means to attain their goals, the list of which is quite extensive. There can be numerous motivations behind cyber threats as they may be performed by various parties/individuals, such as governments, terrorists, hacktivists, etc. All of them have their proper objectives, the majority of which can belong to some of the common groups: curiosity (most applicable to individual script kiddies), vandalism, hacktivism, industrial espionage, extortion or fraud, and information warfare.
Cyber-attacks are intended for those who prefer to act sleek and stealthy, and thus entities/individuals/governments oftentimes utilize those instead of straight-on physical attacks to act more discretely. The motivation to conduct an attack anonymously is also another factor to bear in mind. In the case of governments this enables them to perform the attack without bearing consequences (if its origin remains undetected) or it can enable them to avoid additional challenges related to international law. In the case of Stuxnet for instance, where there was presumably an immediate need for an intervention in Iran's growing nuclear program, the US and Israel both knew that military action would destabilize the region and incur consequences and retaliation from Iran and thus chose to employ digital means instead.
However, some parties, terrorist groups, for instance, may employ classical methods of combat. Blowing something off or any other physical attacks do not require sophistication and computer skills in most cases. Furthermore, if the primary goal is to gain attention with an act of some sort, terrorist groups may still prefer to perform a physical attack simply because it is more demonstrative. A bombing or a terror attack would certainly attract much higher attention from both media and the general public than an infiltration into a network of critical infrastructure. Although, one may argue that if significant damage is caused, resulting in say a flood due to a malfunction in a dam’s control system or any other sort of disaster, this would certainly attract as much attention as in the latter case.
Infrastructure that can be targeted includes electrical systems and blackouts; telecommunications services and internet/voice communication, etc. However, as the readings that we covered suggest, there has not yet been such a case, as in the majority of
cases, an attacker cannot perform an attack of such complexity.
The complexity of cyberattacks coupled with the low chance of a successful attack demotivates the terrorists. However, if an attack on critical infrastructure is successful it might as well attract as much attention as physical attacks. Scalability is another parameter that plays a vital role in any cyber-attack. To scale up a physical attack, would require bringing additional troops, and military equipment, which can be extremely troublesome in logistical terms, especially during a battle. Whereas in the case of cyber-attacks, one might argue that scalability is relatively simpler, as it implies the deployment of more computing resources, which can be done quicker than say shipment of additional equipment to the battlefield. This, however, does not imply it is easy in all terms. \\
\hline
\textbf{GPT: }
The cyber-threat landscape is constantly evolving, but some common types of threats include malware, phishing, ransomware, and distributed denial of service (DDoS) attacks. Malware refers to malicious software that can infect a computer or device and allow an attacker to gain access to sensitive information or disrupt operations. Phishing refers to attempts to trick individuals into providing sensitive information, such as passwords or credit card numbers, through fraudulent email or website. Ransomware is a type of malware that encrypts a victim's files and demands payment in exchange for the decryption key. DDoS attacks involve overwhelming a website or network with traffic to disrupt service.
The motivation behind using cyber-attacks instead of physical attacks is often the ability to carry out an attack remotely and with a lower risk of being caught. Cyber-attacks can also be more cost-effective and have a greater potential impact than physical attacks. Additionally, many organizations and individuals have valuable information stored electronically, making it a more attractive target for cybercriminals. Additionally, it is also a way for hackers to disrupt services of a company or government without having a physical presence in the location. \\
\hline
\end{tabular}
\end{table*}
